# Supplementary material for: Gentopia: A Collaborative Platform for Tool-Augmented LLMs
Source: arXiv:2308.04030 source file (2023-08-08)
Supplement: Supplementary file 1 [file appendix.tex]

This is a section in the appendix.
